# Supplementary material for: Many Body Scars as a Group Invariant Sector of Hilbert Space
Source: arXiv:2007.00845 ancillary file (2020-12-02)
Supplement: Supplementary file 1 [file SM.pdf]

# Supplemental Material for "Many Body Scars as a Group Invariant Sector of Hilbert Space"

## I. THE MATRIX EXAMPLE

As a generalization of the model considered in the main text, let us consider the Hilbert space of $N_1 N_2$ fermionic oscillators

$$\{c_{ab}, c^\dagger_{a'b'}\} = \delta_{aa'}\delta_{bb'}, \quad a = 1, \ldots, N_1 \ , \ b = 1, \ldots, N_2 \ . \tag{1}$$

It transforms under the action of the $U(N_1 N_2)$ group and, therefore, under its subgroups $U(N_1) \times U(N_2)$ and $O(N_1) \times O(N_2)$. It may be interpreted as a lattice with $N_1 N_2$ sites and one fermionic degree of freedom per site. The mapping of the group indices to the spatial lattice sites is again a matter of preference; the simplest choice is that of a rectangular 2D lattice with spinless or spin-polarized fermions. The scars are invariant under the group $G = SU(N_1) \times SU(N_2)$ or $G = SO(N_1) \times SO(N_2)$, corresponding to the choice of complex or imaginary hopping strength, respectively. For the former choice, the invariant subsector consists of only two states, the vacuum and antivacuum. Therefore, we will adopt $G = SO(N_1) \times SO(N_2)$ where the scar sector is much richer. Here the hopping terms are linear combinations of the basis generators of $G$:

$$Q_1^{aa'} = i(c^\dagger_{ab}c_{a'b} - c^\dagger_{a'b}c_{ab}) \ , \ Q_2^{bb'} = i(c^\dagger_{ab}c_{ab'} - c^\dagger_{ab'}c_{ab}) \ .$$

The hoppings describing free electrons are now in both directions with periodic boundary conditions

$$T_a = tQ_1^{a,a+1}, \ T_b = tQ_2^{b,b+1}, \ T = \sum_a T_a + \sum_b T_b \ . \tag{2}$$

As $H_0$ we use a generalization of (3) in the main text:

$$H_0 = 2g\left(c^\dagger_{ab}c^\dagger_{ab'}c_{a'b}c_{a'b'} - c^\dagger_{ab}c^\dagger_{a'b}c_{ab'}c_{a'b'}\right) + 2g(N_2 - N_1)Q + \frac{g}{2}N_1 N_2 (N_2 - N_1) \ , \tag{3}$$

that is also integrable [1, 2] with integer energies in units of $g$ (like in the main text we add $Q$ to split degenerate singlets). The matrix model (3) has a 't Hooft large $N$ limit where $N_1 = N_2 = N$ is sent to infinity while keeping $gN$ fixed. The $H_0$ used in the main text case is related to the vector large $N$ limit where $N_2 = 2$, while $N_1 = N$ is sent to infinity keeping $gN$ fixed [1, 2] (we set $g = 1$ in the main text). For these reasons we refer to the examples considered in the main text and SM as vector and matrix respectively.

The full Hamiltonian reads

$$H = H_0 + T + 4\sum_{a,b,b'} O_{a,b,b'}T_a + 4\sum_{a,a',b} O_{a,a',b}T_b, \tag{4}$$

where

$$O_{a,b,b'} = q_{a,b,b'}c^\dagger_{(a+3)b}c_{(a+3)b'} + p_{a,b,b'}c^\dagger_{(a+3)b}c^\dagger_{(a+3)b'} + \text{h.c.}$$

$$O_{a,a',b} = r_{a,a',b}c^\dagger_{a(b+2)}c_{a'(b+2)} + s_{a,a',b}c^\dagger_{a(b+2)}c^\dagger_{a'(b+2)} + \text{h.c.},$$

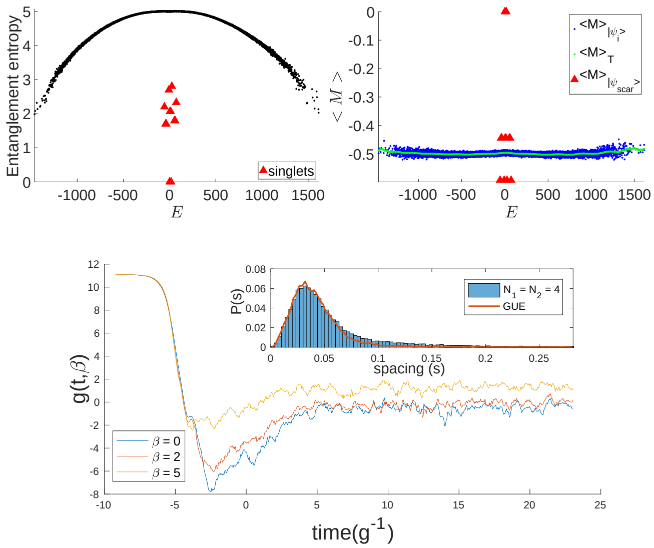


FIG. 1. Matrix model (I) with $N_1 = N_2 = 4$. Top left panel: Entanglement entropy; Top right panel: ETH plot for the diagonal hopping $M = (c^\dagger_{11}c_{22} - c^\dagger_{22}c_{11})^2$; Bottom: Nearest neighbor eigenvalue spacings (inset) and the spectral form factor for the 442 model

with $q, p, r, s$ random complex numbers.

Numerical results for $N_1 = N_2 = 4$ and $t = 8\sin\sqrt{2}\pi$ are shown in Fig. 1 and similarly to the vector case demonstrate that the $G = SO(N_1) \times SO(N_2)$-invariant states become scars.

The more complex structure of singlets is reflected in the fact that, unlike in the vector case, only the trivial states (the vacuum $|0\rangle$ and antivacuum $|1\rangle$) have zero entropy and are product states. The following operators may be used (see Sec. III and [1]) to construct the complete sets of scars in the sense that their linear combinations and products acting on $|0\rangle$ span the full singlet subspace $\mathbb{S}$

$$(J_+)_{aa'} = c^\dagger_{ab}c^\dagger_{a'b}, \quad (K_+)_{a_1\ldots a_{N_1}} = \epsilon_{b_1\ldots b_{N_2}}\prod_{i=1}^{N_{1/2}} c^\dagger_{a_i b_i},$$

where indices of $J_+, K_+$ should be contracted with the use of $\delta_{aa'}$ or the $(J^n_+)_{aa'}$. For $N_{1,2} = 2$, $K_+$ corresponds to the $\eta$-pairing of the Hubbard model. Because they are singlets, these states again possess the ODLRO as we prove in Sec. IV. The structure of the states is much more complex than in the vector case. The long-range order in the language of ref. [3] is described, in part, as a mix of two types: $G_O$, superconducting in one direction while magnetic in the other and $G_U$, magnetic in both directions. In the finite-size system we find numerically (see fig. 5) that the following correlator is non-vanishing for all non-trivial scars $|s\rangle$: $G_O(a_{1,2}, b_{1,2}) = \langle s|c^\dagger_{a_1b_1}c^\dagger_{a_1b_2}c_{a_2b_2}c_{a_2b_1}|s\rangle$, and is so even at large separations in the $a$ direction, corresponding to the superconducting phase, while in the $b$ direction we would get particle-hole

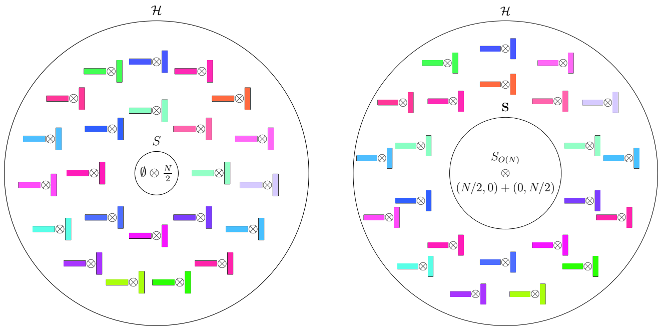


FIG. 2. Graphical view of the two ways to factorize the Hilbert space considered in the main text. Each colour visualises a different representation. The center represents a singlet subspace. The horizontal bar corresponds to the young tableaux of the $U(N)$ group, while the vertical ones to $U(2)$ — showing the connection that to go from one group to the other one should transpose the corresponding Young Tableaux.

pairs. Further examples of ODLRO that we find numerically lack a simple interpretation in terms of $G_O$ and $G_U$; they are $\langle s|c^\dagger_{11}c^\dagger_{1N_2}c_{N_1N_2}c_{N_11}|s\rangle$ and $\langle s|c^\dagger_{11}c_{1N_2}c^\dagger_{N_1N_2}c_{N_11}|s\rangle$.

In contrast to the vector case, the dimension of the scar subspace grows exponentially with $N_1N_2$ [1]; nevertheless, it spans only an exponentially small fraction of the Hilbert space. It is conceivable that for large $N_1N_2$ the scar states may form continuous energy bands filled with the states possessing ODLRO.

## II. HOPPING AMPLITUDES AND GENERATORS

Let us study the Hermitian bilinear operators which preserve charge $Q$,

$$T_A = \sum_{a,a',b} A_{aa'}c^\dagger_{ab}c_{a'b}, \quad A^\dagger = A\,. \tag{5}$$

Their commutation relations are

$$[T_A, T_B] = T_{[A,B]}\,. \tag{6}$$

If we further require $A$ to be traceless, this is isomorphic to the $SU(N)$ algebra.

Each subalgebra of $SU(N)$ corresponds to a subalgebra of (5) and vice versa. For example, we can take an algebra of antisymmetric matrices $O(N) \subset SU(N)$—they would correspond to the hoppings with purely imaginary amplitudes. It is generated as a Lie algebra by the nearest-neighbor hoppings

$$T_a = ic^\dagger_{ab}c_{(a+1)b} + \text{h.c.}\,, \tag{7}$$

which form a maximal subalgebra of $SU(N)$.

Another interesting example of subalgebra arises for the real nearest-neighbor hoppings

$$\tilde{T}_a = c^\dagger_{ab}c_{(a+1)b} + \text{h.c.} \tag{8}$$

Let $\mathfrak{g} \subset \mathfrak{su}(N)$ be a minimal Lie algebra containing $\tilde{T}_a$. One can see that when $N$ is even we can make a transformation $c_{2a,b} \to ic_{2a,b}$ that would send $\tilde{T}_a$ to $T_a$. Hence we get $\mathfrak{g} \approx \mathfrak{o}(N)$, but it is a different embedding of the original $O(N)$ mentioned before. This trick also could be used on the bipartite lattices — the lattices where all sites could be separated into two groups, and the edges connect vertices from different sets.

In this case the family of the invariant states for this group looks like the usual $\eta$-pairing states [4]

$$|n'_O\rangle = \frac{\left(\sum_a e^{i\pi a}c^\dagger_{a1}c^\dagger_{a2}\right)^n}{\sqrt{\frac{N!n!}{(N-n)!}}}|0\rangle\,. \tag{9}$$

For odd $N$ one can show that $\tilde{T}_a$ will comprise the full algebra $\mathfrak{su}(N)$.

One can consider index $b$ as a lattice index. Therefore we could associate another group $U_b(N)$ with generators

$$T_b = \sum_{a,b,b'} B_{b,b'}c^\dagger_{ab}c_{ab'}. \tag{10}$$

Then combining these two generators we get that the $U(N_1)\times U(N_2)$ group acts in the Hilbert space, and it could be used as group $G$ in the general construction studied in the main text. However, there are only two $U(N_1)\times U(N_2)$ invariant states [5]. To get richer structure we consider only the hoppings with purely imaginary amplitudes leading to $O(N_1)\times O(N_2)$.

We can also generalize $T$ to be not only a nearest-neighbor hopping but to be any hopping in the lattice. It allows us to deform the vector model to be not only a 1D lattice, but an arbitrary dimensional lattice. For example, we can consider a 3D Hubbard model. The fermion operators have 4 index: $c_{xyz,\sigma}$ where $x,y,z = 1,\dots,L$ are lattice coordinates. We can rearrange them into a linear index as $i = x+(y-1)*L+(z-1)*L^2$. Then the hoppings from $i$ to $i+1$ correspond to $x$-directed hoppings, $i$ to $i+N$ is a $y$-directed hopping, and from $i$ to $i+N^2$ is a $z$-directed hopping. Any of these hoppings are the generators of $U(N=L^3)$ and therefore the reasoning presented above would still work for this case.

We end this subsection with a derivation of the structure of the term $H_1$ in our Hamiltonian. Let us take a Hilbert space with the action of some Lie algebra $\mathfrak{g}$ realized by some hermitian operators. Let $T_i$ be a simple basis of the generators of this algebra $\mathfrak{g}$, meaning that whole algebra is spanned by $T_i$ and all of their possible commutators. Let $\mathbb{S}$ be a space of invariant states $\mathfrak{g}\mathbb{S} = 0$. Then if $K$ is an annulator of $\mathbb{S}$, *i.e.* $K\mathbb{S} = 0$; then $K = \sum_j O_jT_j$.

The proof is quite simple. We introduce operator $C = \sum T_i^2$—it is an annulator of $\mathbb{S}$ since $Cv = 0 \Leftrightarrow T_iv = 0 \Leftrightarrow v \in \mathbb{S}$. We can define $C^{-1}$ such that $C^{-1}\cdot C = 1 - P_{\mathbb{S}}$, where $P_{\mathbb{S}}$ is a projector on $\mathbb{S}$ and therefore $C^{-1}\cdot C$ is also an annulator of $\mathbb{S}$. Then

$$K = K(1-P_{\mathbb{S}}) = \\ = K\cdot C^{-1}\cdot C = \sum_i (K\cdot C^{-1}\cdot T_i)T_i = \sum_i O_iT_i\,, \tag{11}$$

as required

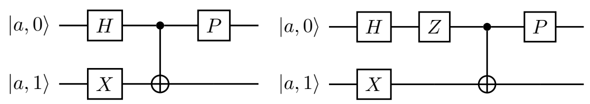


FIG. 3. Left panel: Circuit diagram of $W_a$ for construction of $|S_1\rangle$ states (6). $H$ is the Hadamard gate, $X$ is the Pauli-X gate, the line spanning the two sites represents the CNOT gate from qubit 0 to target qubit 1, and $P$ is the phase gate. Right panel: Circuit diagram of $\tilde{W}_a$ gates needed to construct the singlet state $|S_2\rangle$.

## III. CONSTRUCTION OF GROUP INVARIANT STATES

The two states $|S_{1,2}\rangle$ (6) with zero entanglement entropy may be expressed as a product state with the use of the gates $W_a$ and $\tilde{W}_a$ (see fig. 3):

$$|S_1\rangle = \prod_{a=1}^{N} W_a |0\rangle \,, \quad |S_2\rangle = \prod_{a=1}^{N} \tilde{W}_a |0\rangle \qquad (12)$$

Let us also present another, rotated basis for the family of states (7), which are $U(N)$ invariant and transform as spin $N/2$ under the rotational $SU(2)$ symmetry:

$$|\tilde{n}_U\rangle = \frac{\left(\sum_a c^\dagger_{a1} c_{a2}\right)^n}{2^n \sqrt{\frac{N!n!}{(N-n)!}}} |\tilde{S}_2\rangle \,, \qquad (13)$$

with $n = 0, \ldots, N$. Here

$$|\tilde{S}_1\rangle = \prod_{a=1}^{N} c^\dagger_{a1} |0\rangle \quad , \qquad |\tilde{S}_2\rangle = \prod_{a=1}^{N} c^\dagger_{a2} |0\rangle \quad . \qquad (14)$$

For the Hamiltonian $H_0$ in (3), the states $|\tilde{n}_U\rangle$ are not eigenstates, while the states $|n_U\rangle$ given in (7) are. However, for the Fermi-Hubbard and Heisenberg models, which respect the $SU(2)$ rotational symmetry, both $|\tilde{n}_U\rangle$ and $|n_U\rangle$ are eigenstates.

As shown in the main text, some singlet states in the vector model are related to the $\eta$-pairing states discovered by Yang [6]. We can extend this construction to the matrix model that was discussed in [1]. We start with the vacuum state $|0\rangle$ that is naturally a singlet state, because it is annihilated by any hopping. Then in order to build any other singlet state we can act with the creation operator and pair the index with the use of the $\delta$ - pairing or $\epsilon$ - pairing. Namely, we introduce

$$(J_+)_{aa'} = c^\dagger_{ab} c^\dagger_{a'b}, \quad (K_+)_{a_1 \ldots a_{N_1}} = \epsilon_{b_1 \ldots b_{N_2}} \prod_{i=1}^{N_{1/2}} c^\dagger_{a_i b_i}.$$

These operators automatically are singlets under the action of $SO_b(N)$. Then the singlet states could be constructed out of the products and sums of the operators $J_+$, $K_+$ by contracting indices with the use of $\delta_{aa'}$ or $\epsilon_{a_1 \ldots a_N}$.

The states with a small number of fermions could be built with the use of only the operator matrix $J_+$. We introduce

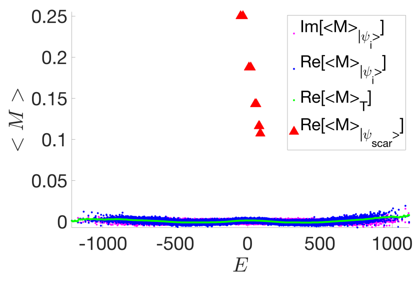


FIG. 4. Correlator $G_U = \langle c^\dagger_{11} c_{12} c^\dagger_{42} c_{41}\rangle$ (see (19)) evaluated for every eigenstate of the vector model with $N = 8$. All $9 = N + 1$ states $|n_U\rangle$, defined in (7), exhibit the "magnetic" ODLRO. The value of $G_U$ for this family of scar states is $G_U = \frac{1}{4} - \frac{n(N-n)}{2N(N-1)}$ and is purely real.

$\mathcal{M}_n = \sum_a (J^n_+)_{aa}$, which is a singlet under the action of $SO_a(N) \times SO_b(N)$. For example, acting with $\mathcal{M}_n$ and their products we can build singlet states as

$$|s_1\rangle = \mathcal{M}_2 |0\rangle \,, \; |s_2\rangle = \mathcal{M}_3 |0\rangle \,, |s_3\rangle = \mathcal{M}_3 \mathcal{M}_4 \mathcal{M}_2^2 |0\rangle \,, \ldots$$

When the number of fermions is larger than $N$, we can use $K_+$ to build singlet states. For example, when $N$ is even we can have

$$|s_\epsilon\rangle = (K_+)_{a_1 a_1 \ldots a_{N/2} a_{N/2}} |0\rangle \,.$$

For $N = 2$ the operator $(K_+)_{aa}$ is the $\eta$-operator from [6].

In general we are able to express the dimension of the singlet subspace as an integral [1]

$$\dim \mathbb{S}_O =$$
$$= \frac{4^{N_1 N_2}}{V_{N_1} V_{N_2}} \int_{-\pi}^{\pi} \prod_{i,j=1}^{N_1,N_2} dx_i dy_j \left(\cos x_i + \cos y_j\right)^2 \times$$
$$\times \prod_{i \neq i'}^{N_1} \left(\cos x_i - \cos x_{i'}\right)^2 \prod_{i \neq i'}^{N_2} \left(\cos y_i - \cos y_{i'}\right)^2 , \qquad (15)$$

where $V_{N_1,N_2}$ are the dimensions of the $SO(N)$ groups, which are equal to

$$V_{N_1} = \int_{-\pi}^{\pi} \prod_i^{N_1} dx_i \times \prod_{i \neq i'}^{N_1} \left(\cos x_i - \cos x_{i'}\right)^2 . \qquad (16)$$

## IV. OFF-DIAGONAL LONG RANGE ORDER (ODLRO)

Let us show that the singlet states $|s\rangle \in \mathbb{S}$ exhibit the Off-Diagonal Long Range Order (ODLRO) [4]. This means that the correlator

$$G_O = \langle s | c^\dagger_{i1} c^\dagger_{i2} c_{j2} c_{j1} | s\rangle \;, \qquad (17)$$

does not depend on $i$ and $j$ when they take different values. Indeed, there is an operator $O_{ik} \in O(N)$ which swaps the

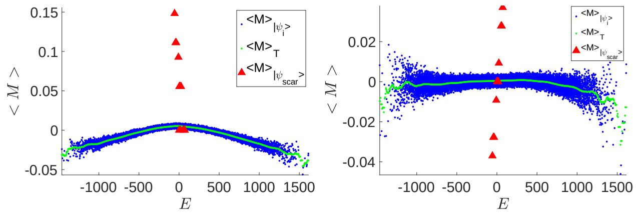


FIG. 5. Left panel: Correlator $G_O = \langle c^\dagger_{11} c^\dagger_{12} c_{42} c_{41} \rangle$ evaluated for every eigenstate of the matrix model with $N = 4$; 7 out of 12 scars have non-vanishing "superconducting" ODLRO. Right panel: Correlator $G_U = \langle c^\dagger_{11} c_{12} c^\dagger_{42} c_{41} \rangle$ evaluated for every eigenstate of the matrix model; 8 out of 12 scars have non-vanishing "magnetic" ODLRO. One can show that $G_O$ and $G_U$ are rational numbers which depend linearly on the $SU(N)$ Casimirs of the scar states.

fermions with indices $i$ and $k$ leaving the others unchanged. For example,

$$O_{ik} c_{i1} O^{-1}_{ik} = c_{k1} , \quad O_{ik} c_{k1} O^{-1}_{ik} = c_{i1} , \quad O_{ik} c_{j1} O^{-1}_{ik} = c_{j1} \, .$$

Since $|s\rangle$ is an $O(N)$ invariant state, we have $O_{ik} |s\rangle = |s\rangle$. Using these relations, we see that the correlator $G_O$ does not depend on the positions of $i \neq j$. Indeed,

$$G_O = \langle s | c^\dagger_{i1} c^\dagger_{i2} c_{j2} c_{j1} | s \rangle = \langle s | O^{-1}_{ik} c^\dagger_{i1} c^\dagger_{i2} c_{j2} c_{j1} O_{ik} | s \rangle = \\ = \langle s | c^\dagger_{k1} c^\dagger_{k2} c_{j2} c_{j1} | s \rangle \; . \tag{18}$$

Hence, it is non-vanishing even when the difference between $i$ and $j$ is large. An analogous argument can be applied to the correlator

$$G_U = \langle s | c^\dagger_{i1} c_{i2} c^\dagger_{j2} c_{j1} | s \rangle \, , \tag{19}$$

when $|s\rangle$ is a $U(N)$ invariant state, demonstrating ODLRO. We note that $G_O$ is the correlator originally used by Yang [6]. It is related to superconductivity, while $G_U$ is related to the magnetic properties of the system.

For matrix models we also have correlators $G_{O,U}$, where we extend the second index to label spatial coordinates along the other direction. One can notice that $G_O$ now plays a double-role: in one direction it is related to the superconducting properties (since if we separate $G_O$ along the direction $a$, it splits into a product of local cooper pair creation operators) and in the other direction it is related to the magnetic properties(since in the direction $b$ the $G_O$ splits in the product of particle-hole creation operators). The correlator $G_U$ is related to the magnetic properties of the states, because in each of the directions it splits into the product of creation and annihilation operators. And again, using the properties of the singlet states, we can interchange indices while the singlet states are left unchanged and we get that the singlet states must have the ODLRO (see fig.5).

## V. DETAILS OF THE NUMERICAL CALCULATIONS OF TIME EVOLUTION

Fig. 7 details the composition of the initial state for time evolution calculation for the vector model. Exact revivals to

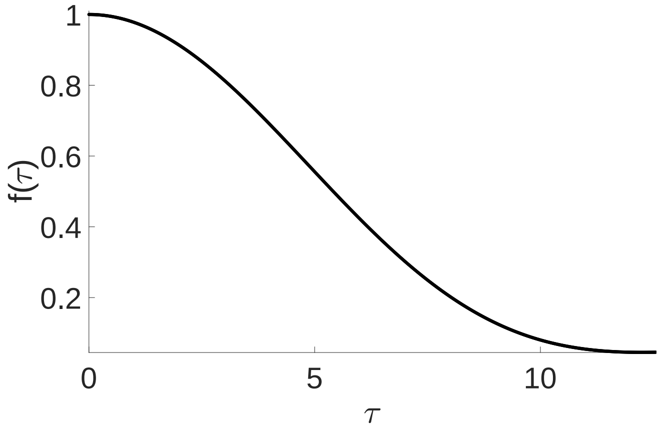


FIG. 6. Time dependence of the fidelity $f(\tau)$ for vector model with $N = 8$. The initial state is a linear combination of 50 eigenstates of $H$ and $\alpha = \sum_{n=1}^{9} |c_n|^2 = 0.95$. The initial state is dominated by 9 generic high-energy states, the fidelity is quickly decaying. The initial state composition for both cases is detailed in fig. 7 and late time behaviour in fig. 8

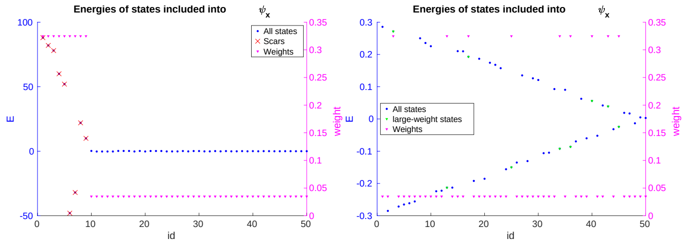


FIG. 7. Initial state composition for the time evolution of the vector model. For every state included into the initial state we plot its ID ($x$ axis), energy and weight in the initial wavefunction ($y$ axes). In both cases the initial state is a mix of 50 eigenstates of $H$ with 9 dominant states contributing 0.95 of the wavefunction norm. Remaining 39 states are generic states from the middle of the spectrum. The two scenarios we are considering are when the dominant states are scar states (top panel) or generic states near $E = 0$ (bottom panel).

$f^{max}(\tau) = 1$ would occur for an initial state comprised solely of scars. Instead, we admix 5 percent of generic states to analyze the stability of the effect in an (experimental) scenario when the desired initial state can only be created with a finite precision.

Fig. 8 shows the time evolution at late times where in presence of scars, the revivals continue with stabilized amplitude and all information is lost without scars.

[1] Igor R. Klebanov, Alexey Milekhin, Fedor Popov, and Grigory Tarnopolsky, "Spectra of eigenstates in fermionic tensor quantum mechanics," Phys. Rev. **D97**, 106023 (2018),

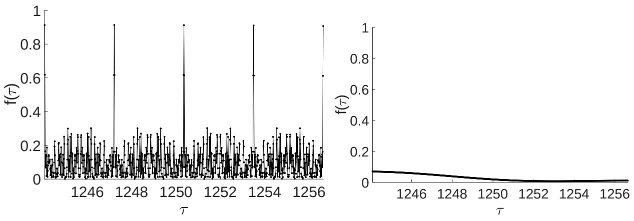


FIG. 8. Time evolution for the vector model at late times. The amplitudes of revivals stabilize at the expected value $\approx 0.95^2$ with scars present (left panel). No revivals occurs when the initial state did not include scars (right panel)


arXiv:1802.10263 [hep-th].

[2] Gabriel Gaitan, Igor R. Klebanov, Kiryl Pakrouski, Preethi N. Pallegar, and Fedor K. Popov, "Hagedorn Temperature in Large $N$ Majorana Quantum Mechanics," Phys. Rev. D **101**, 126002 (2020), arXiv:2002.02066 [hep-th].

[3] Shoucheng Zhang, "So(4) symmetry of the hubbard model and its experimental consequences," International Journal of Modern Physics B **05**, 153–168 (1991), https://doi.org/10.1142/S0217979291000110.

[4] Chen Ning Yang, "Concept of off-diagonal long-range order and the quantum phases of liquid he and of superconductors," Reviews of Modern Physics **34**, 694 (1962).

[5] Igor R. Klebanov, Fedor Popov, and Grigory Tarnopolsky, "TASI Lectures on Large $N$ Tensor Models," *Proceedings, Theoretical Advanced Study Institute in Elementary Particle Physics: Physics at the Fundamental Frontier (TASI 2017): Boulder, CO, USA, June 5-30, 2017*, PoS **TASI2017**, 004 (2018), arXiv:1808.09434 [hep-th].

[6] Chen Ning Yang, "$\eta$ pairing and off-diagonal long-range order in a hubbard model," Phys. Rev. Lett. **63**, 2144–2147 (1989).
